# Supplementary material for: Real-World Evaluation of Full-Duplex Millimeter Wave Communication Systems
Source: arXiv:2307.10523 source file (2023-07-20)
Supplement: Supplementary file 1 [file sec-appendix.tex]

\appendices

\section{Test}
